# Supplementary material for: Kronecker-factored Quasi-Newton Methods for Deep Learning
Source: arXiv:2102.06737 source file (2022-02-19)
Supplement: Supplementary file 1 [file experiment_not_used.tex]

\subsection{$\pi \neq 1$}

We'd like to compute (or estimate) $\pi := \sqrt{\frac{\overline{\lambda}(A)}{\overline{\lambda}(G)}}$, where $\overline{\lambda}()$ denotes the "average eigenvalue" operator. 

Suppose we have already computed this $\pi$. In K-BFGS, we then compute
\begin{align*}
    H_A \approx \left( A + \pi \sqrt{\lambda} I \right)^{-1},
    \\
    H_G \approx \left( G + \frac{1}{\pi} \sqrt{\lambda} I \right)^{-1}.
\end{align*}
In other words,
\begin{align*}
    H_A^{-1} \approx A + \pi \sqrt{\lambda} I,
    \\
    H_G^{-1} \approx G + \frac{1}{\pi} \sqrt{\lambda} I.
\end{align*}
Taking the $\overline{\lambda}()$ operator on these equations, we have
\begin{align}
    \overline{\lambda}(H_A^{-1}) \approx \overline{\lambda}(A) + \pi \sqrt{\lambda},
    \label{eq_15}
    \\
    \overline{\lambda}(H_G^{-1}) \approx \overline{\lambda}(G) + \frac{1}{\pi} \sqrt{\lambda}.
    \label{eq_16}
\end{align}

% \ref{eq_14}
% \ref{eq_15} no
% \ref{eq_16} no

If we assume $\pi = \sqrt{\frac{\overline{\lambda}(A)}{\overline{\lambda}(G)}}$, we the have
\begin{align*}
    \frac{\overline{\lambda}(H_A^{-1})}{\overline{\lambda}(H_G^{-1})}
    \approx
    \frac{\overline{\lambda}(A) + \sqrt{\frac{\overline{\lambda}(A)}{\overline{\lambda}(G)}} \sqrt{\lambda}}{\overline{\lambda}(G) + \sqrt{\frac{\overline{\lambda}(G)}{\overline{\lambda}(A)}} \sqrt{\lambda}}
    = \frac{\overline{\lambda}(A)}{\overline{\lambda}(G)}
\end{align*}
Hence, we could safely say that $\sqrt{\frac{\overline{\lambda}(H_A^{-1})}{\overline{\lambda}(H_G^{-1})}}$ is an estimator to $\pi$, provided that the $\pi$ used in computing $H_A$ and $H_G$ is already good enough. However, as shown in (\ref{eq_15}) and (\ref{eq_16}), 
\begin{align*}
    \overline{\lambda}(H_A^{-1}) \neq \overline{\lambda}(A),
    % \label{eq_15}
    \\
    \overline{\lambda}(H_G^{-1}) \neq \overline{\lambda}(G),
    % \label{eq_16}
\end{align*}
especially if $\lambda$ is not small.

\subsection{Non-seed results}

\begin{figure}[H]
  \centering
    \includegraphics[width=0.5\textwidth]{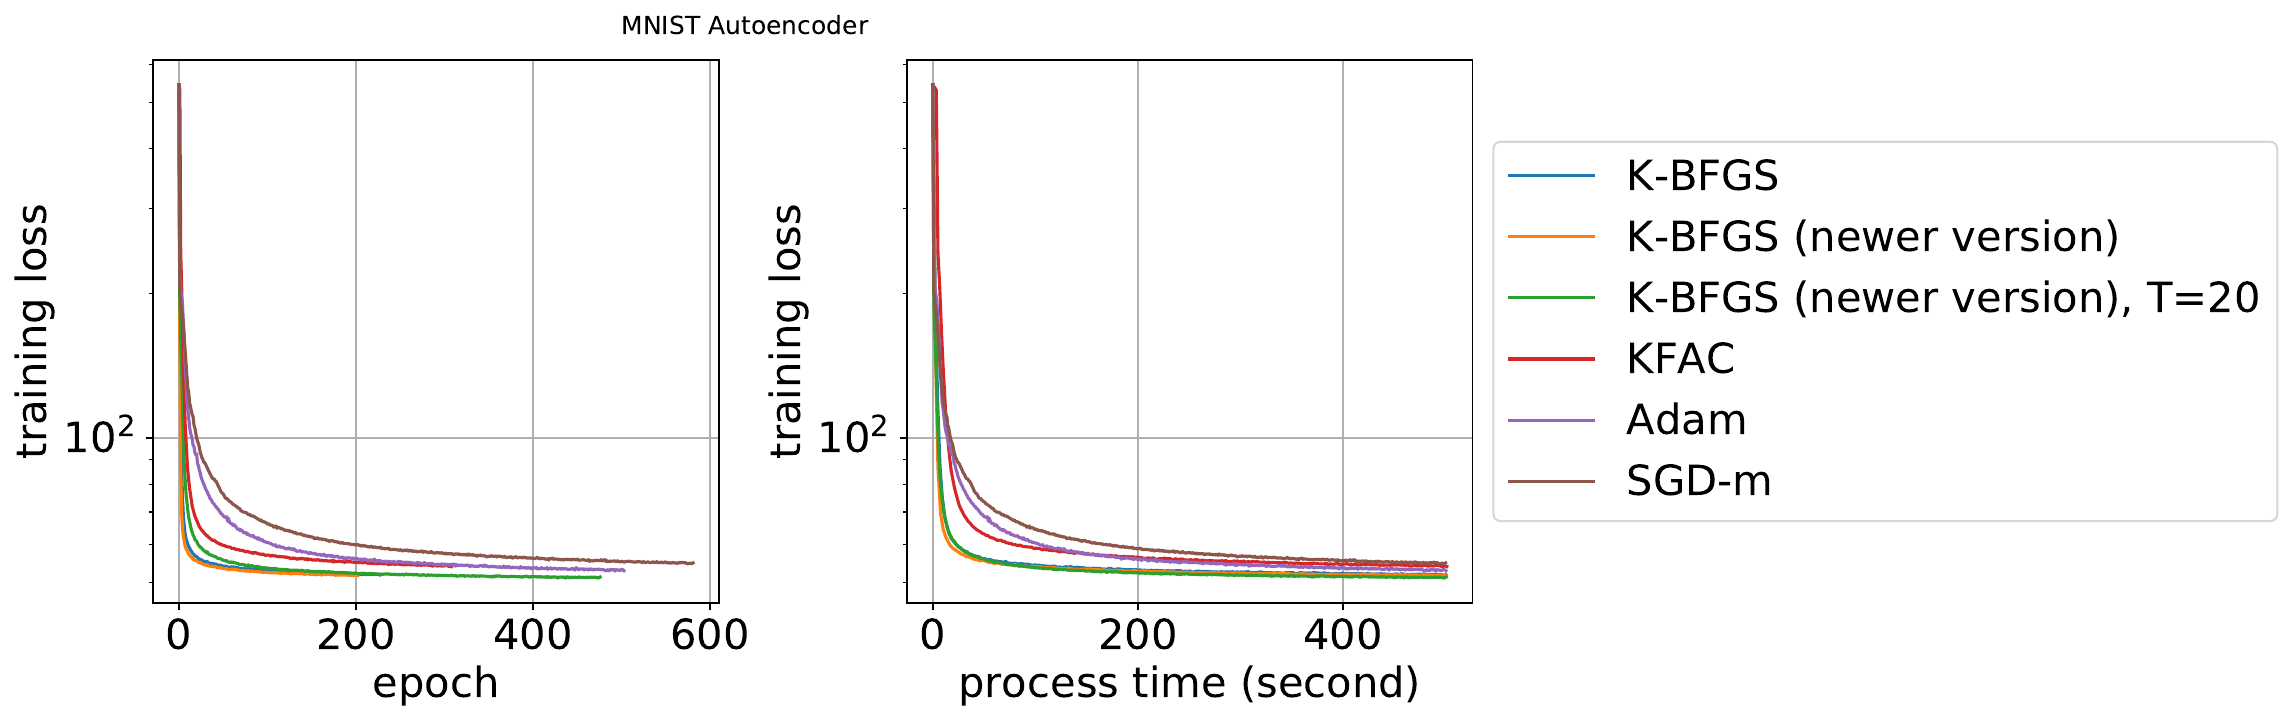}
  \caption{MNIST}
%   \label{fig_33}
\end{figure}

\begin{figure}[H]
  \centering
    \includegraphics[width=0.5\textwidth]{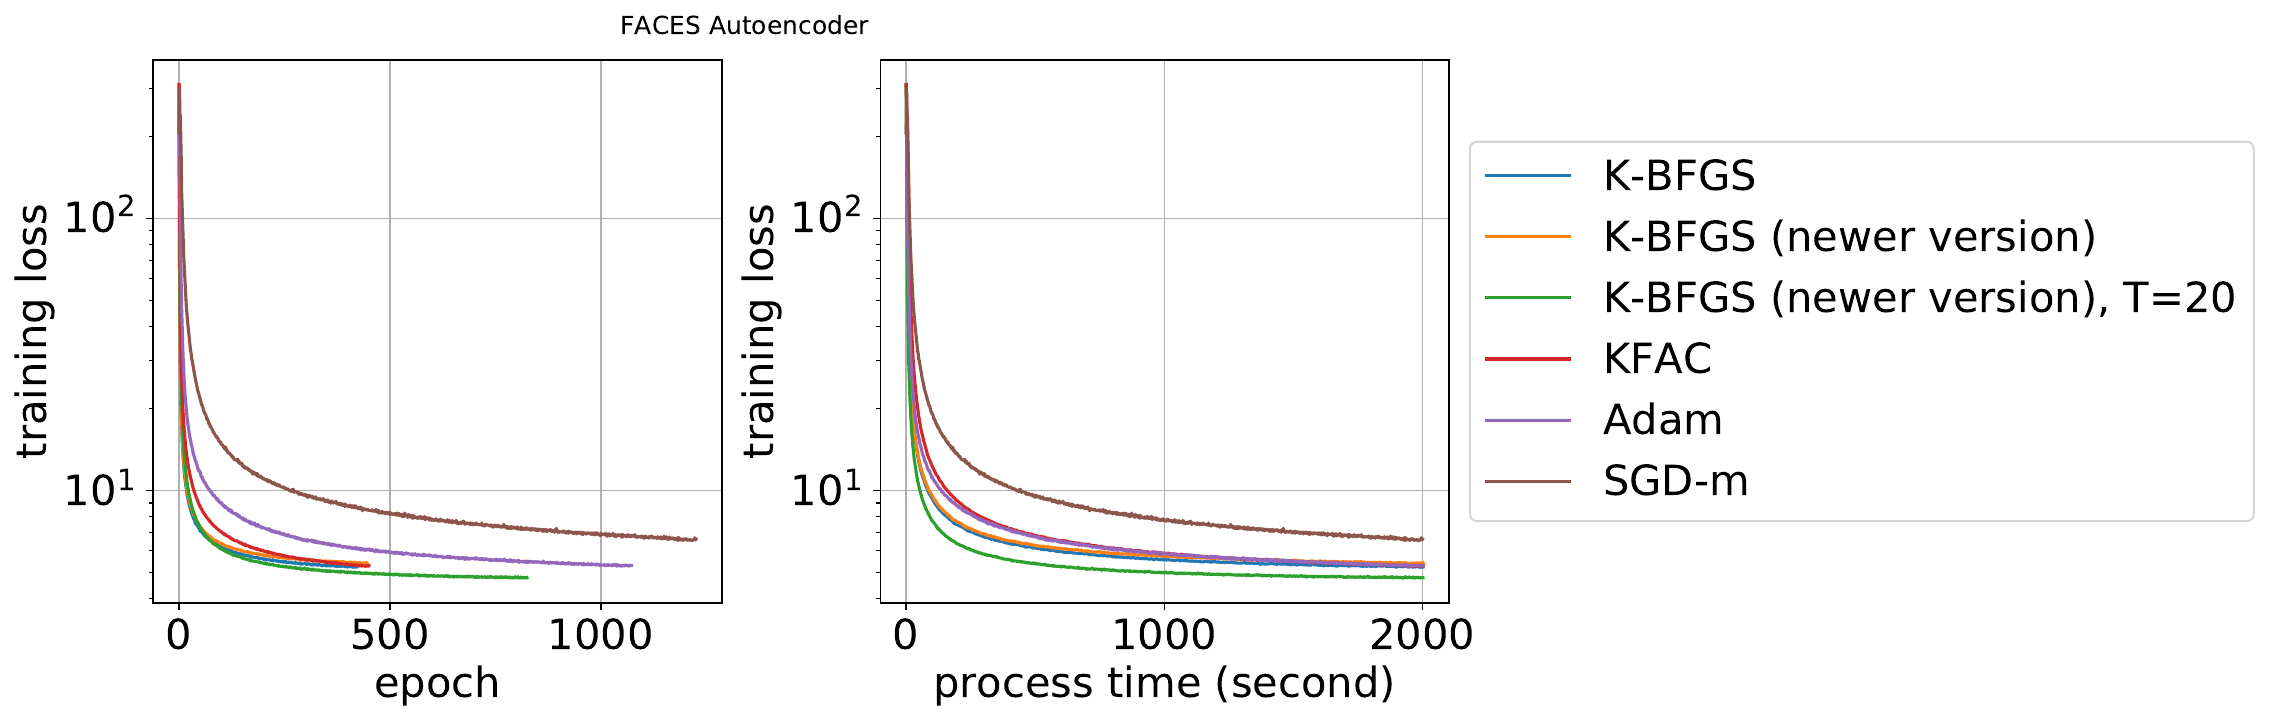}
  \caption{FACES}
%   \label{fig_33}
\end{figure}

\begin{figure}[H]
  \centering
    \includegraphics[width=0.5\textwidth]{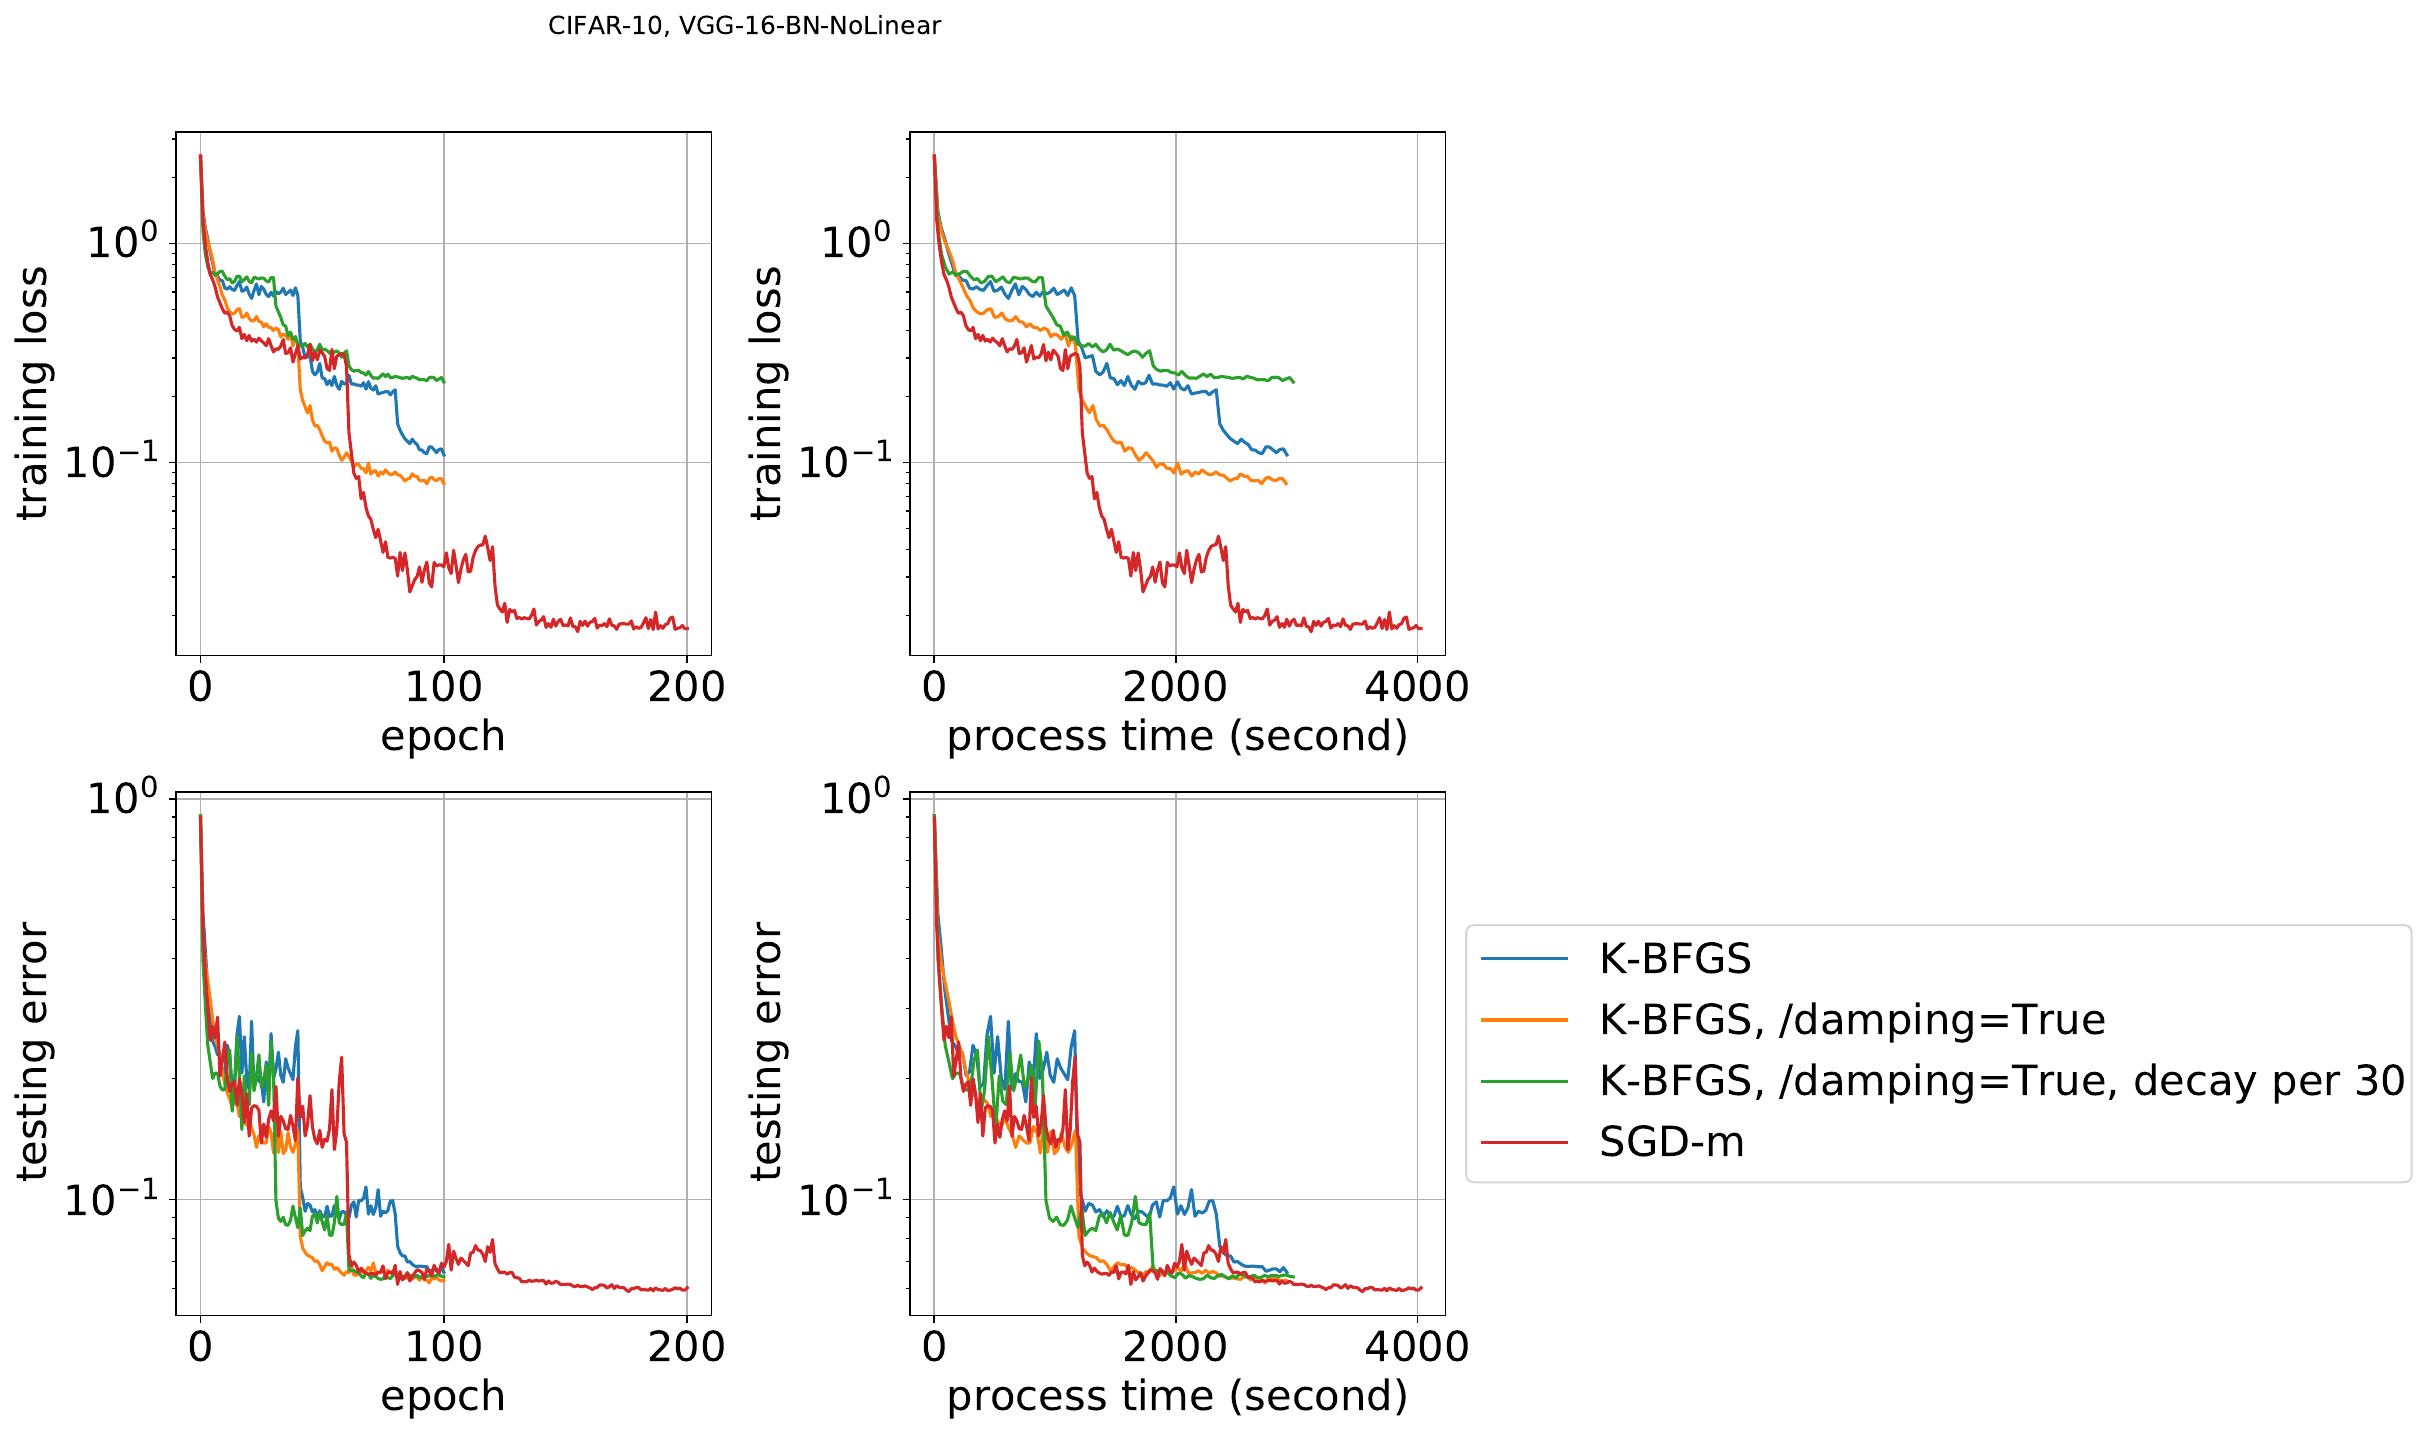}
  \caption{VGG16BN (no large linear layers), CIFAR10}
  \label{fig_2}
\end{figure}

\begin{figure}[H]
  \centering
    \includegraphics[width=0.5\textwidth]{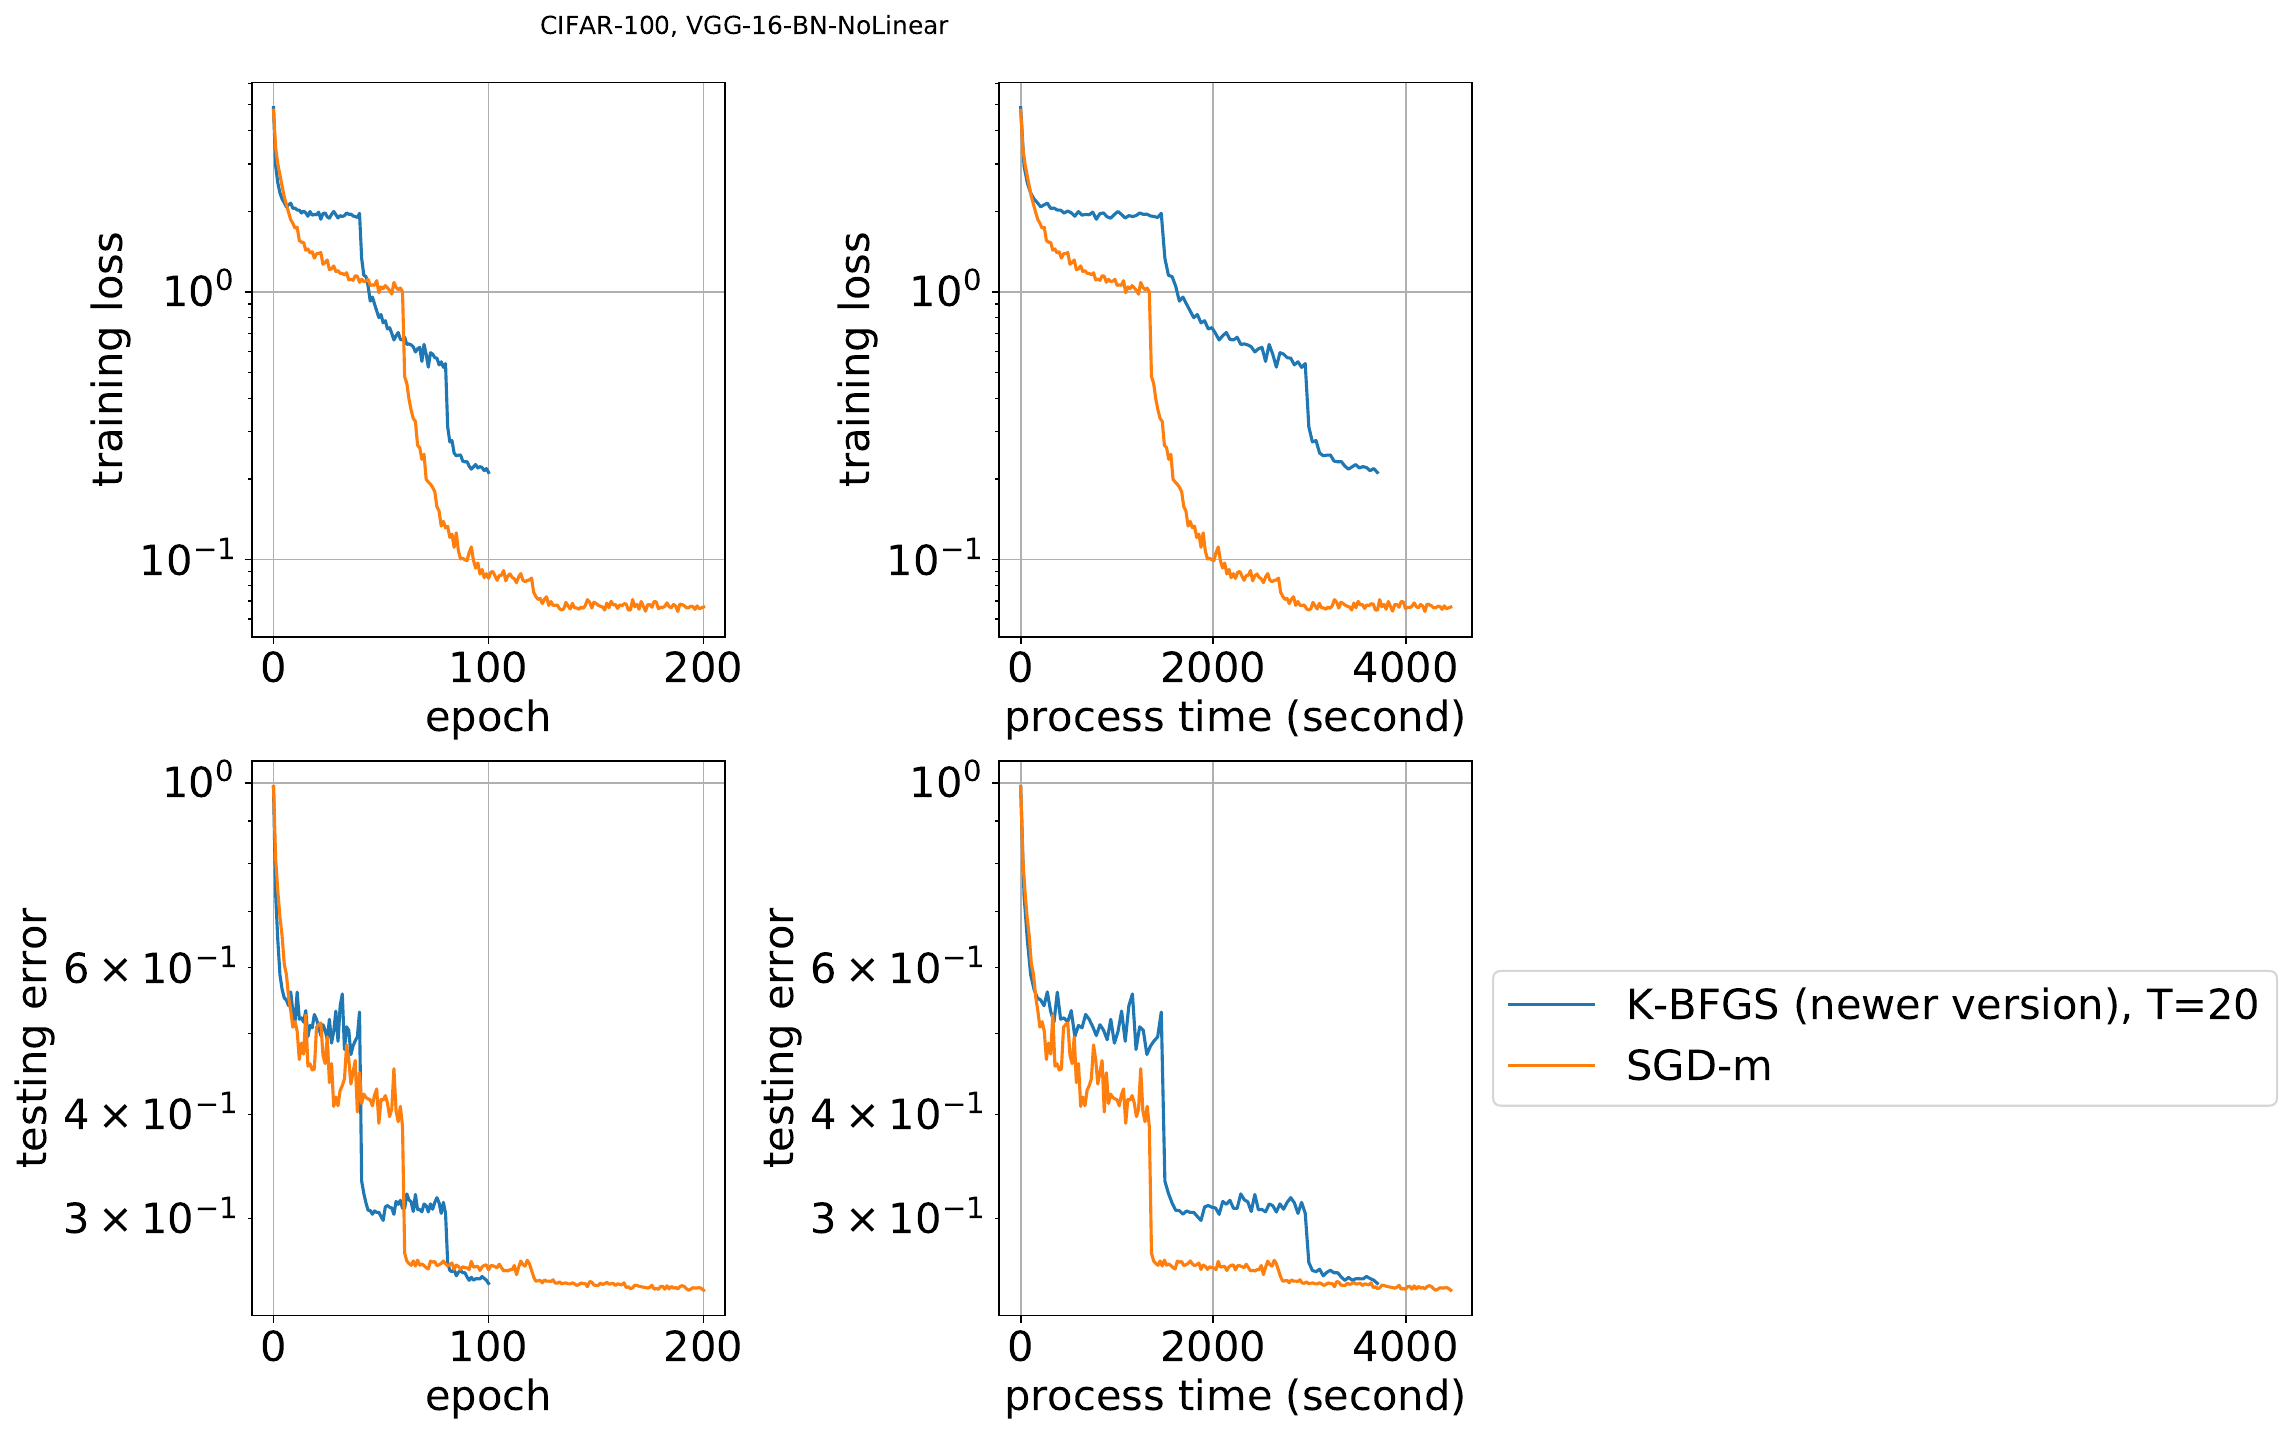}
  \caption{VGG16BN (no large linear layers), CIFAR100}
%   \label{fig_2}
\end{figure}

\begin{figure}[H]
  \centering
    \includegraphics[width=0.5\textwidth]{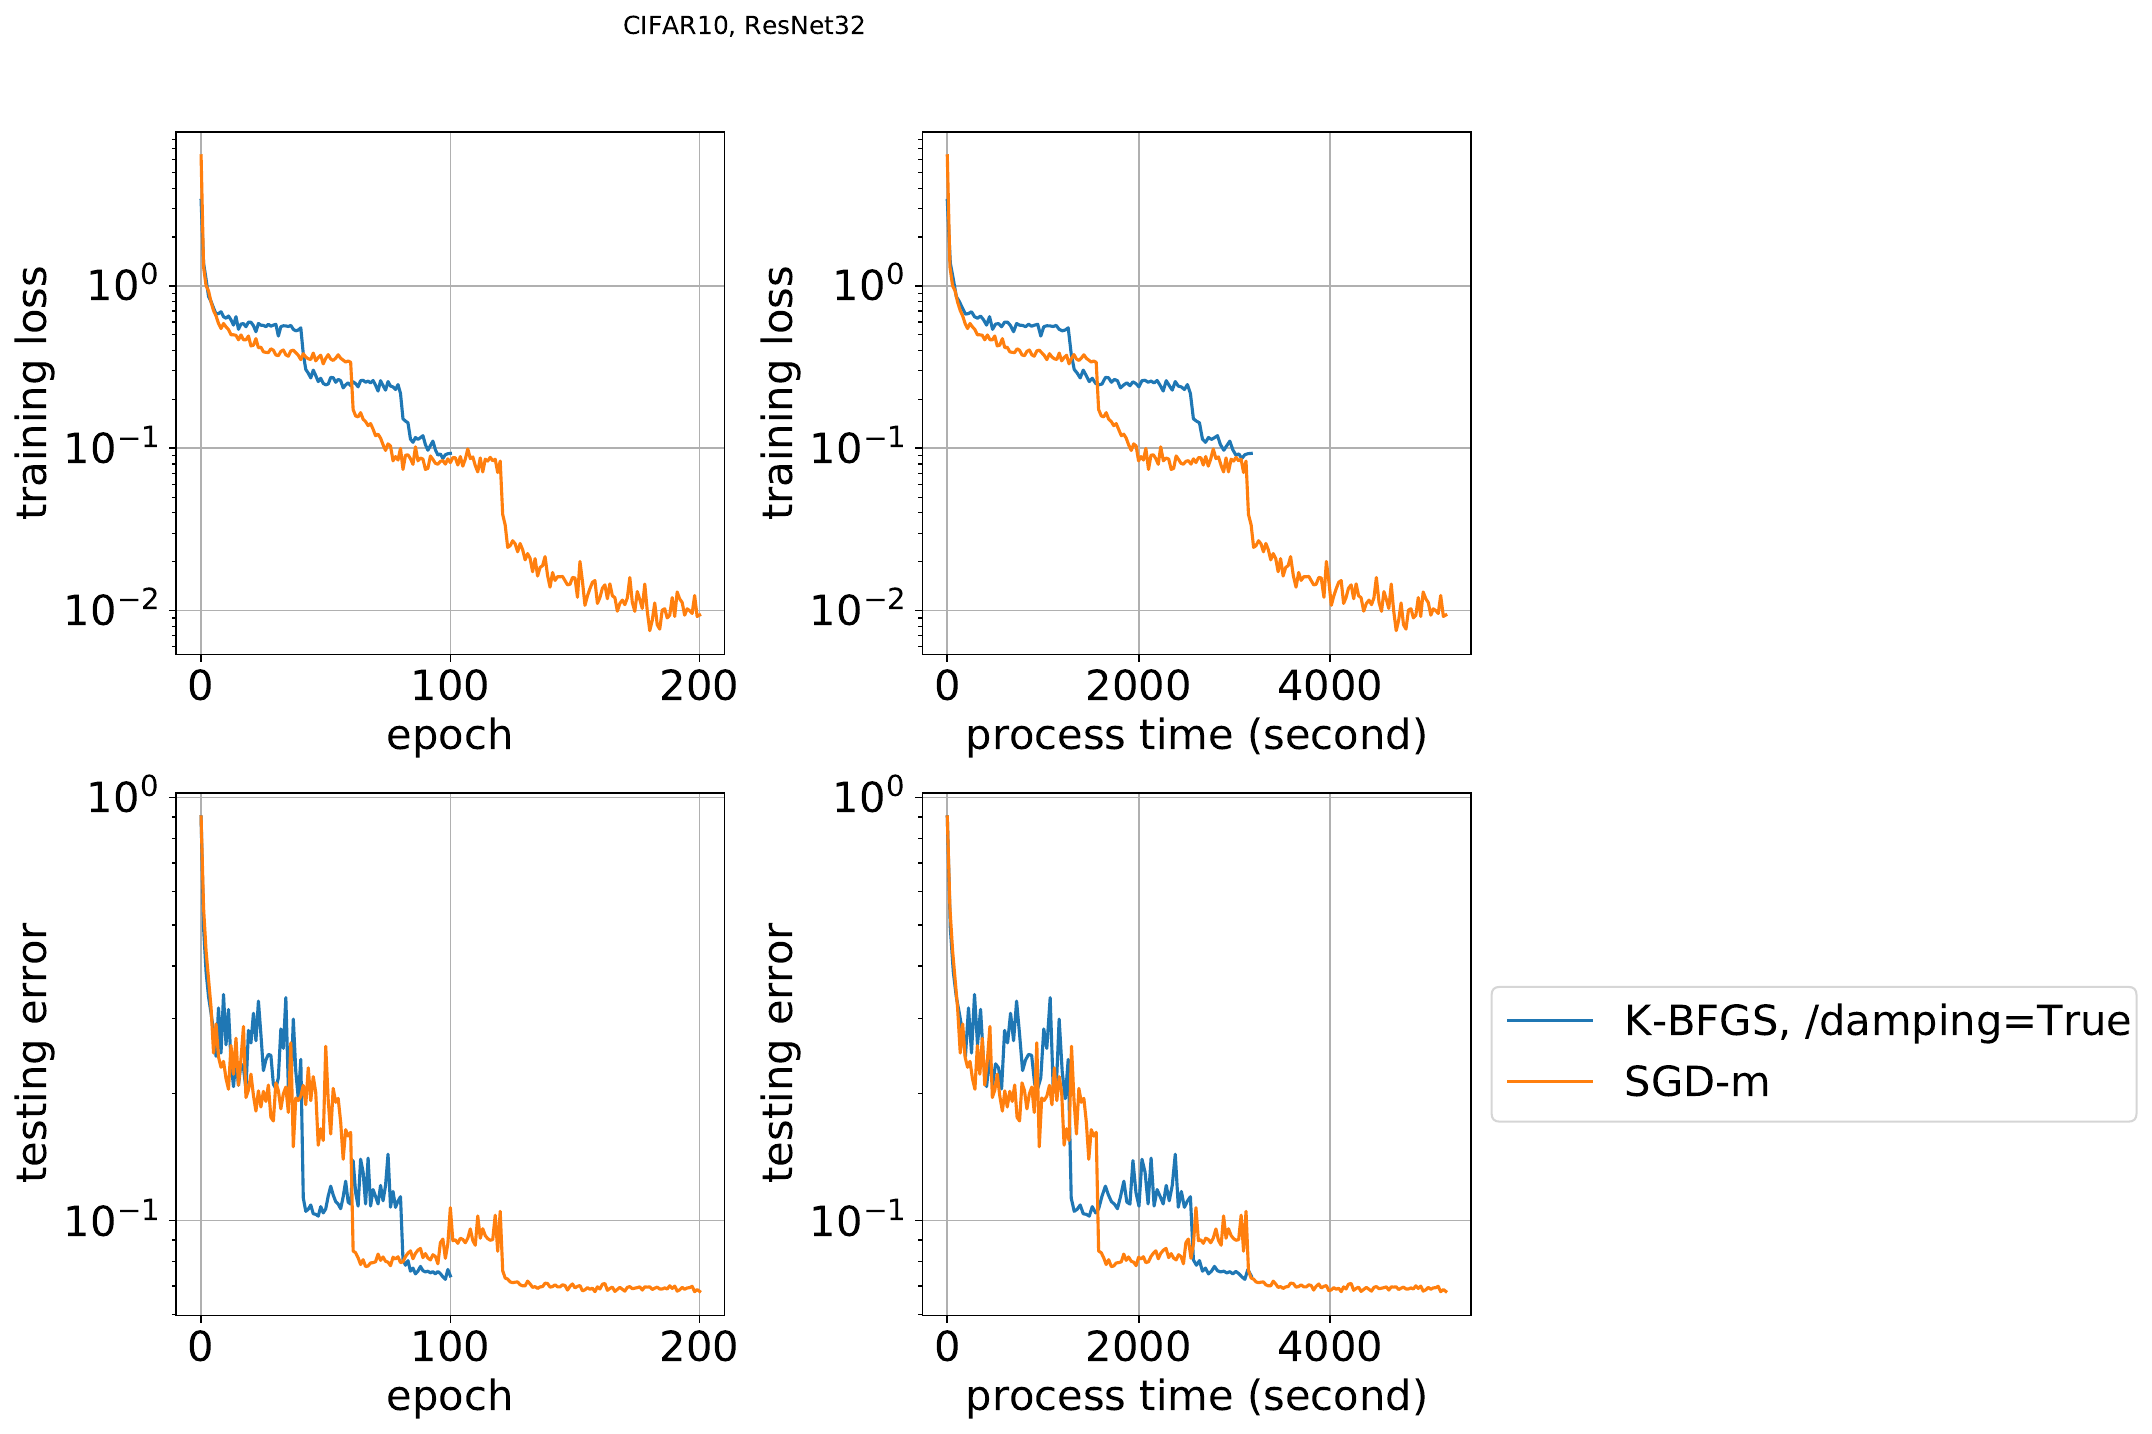}
  \caption{ResNet32, CIFAR10}
%   \label{fig_33}
\end{figure}

\subsection{Stability of KF-QN-CNN}
\label{sec_7}

In Fig \ref{fig_36}, we plot the performance of KF-BFGS-CNN on the same four problems that were used to obtain the results plotted in Figures \ref{fig_33} and \ref{fig_37}, with damping values of $\lambda \in \{ 0.3, 1, 3, 10, 30, 100 \}$ and their corresponding best learning rates. SGD with momentum is also plotted as a baseline. We can see that, in our experiments, KF-BFGS-CNN is not very sensitive to the choice of the damping value when combined with the best learning rate for that choice.

% \begin{figure}[H]
%     \centering
%     \includegraphics[width=0.5\textwidth]{figures/stability/AllCNN-CIFAR10-augmented-0123.pdf}
%     \caption{Stability for All-CNN, augmented CIFAR10}
%     \label{fig_10}
% \end{figure}

% \begin{figure}[H]
%     \centering
%     \includegraphics[width=0.5\textwidth]{figures/stability/VGG16-CIFAR10-augmented-0123.pdf}
%     \caption{Stability for VGG16, augmented CIFAR10}
%     \label{fig_11}
% \end{figure}

% \begin{figure}[H]
%     \centering
%     \includegraphics[width=0.5\textwidth]{figures/stability/AllCNN-CIFAR100-augmented-0124.pdf}
%     \caption{Stability for All-CNN, augmented CIFAR100}
%     \label{fig_34}
% \end{figure}

% \begin{figure}[H]
%     \centering
%     \includegraphics[width=0.5\textwidth]{figures/stability/VGG16-CIFAR100-augmented-0124.pdf}
%     \caption{Stability for VGG16, augmented CIFAR100}
%     \label{fig_35}
% \end{figure}

\begin{figure*}
  \centering
  \begin{minipage}[b]{0.49\textwidth}
    \centering
    \includegraphics[width=\textwidth, height=7cm]{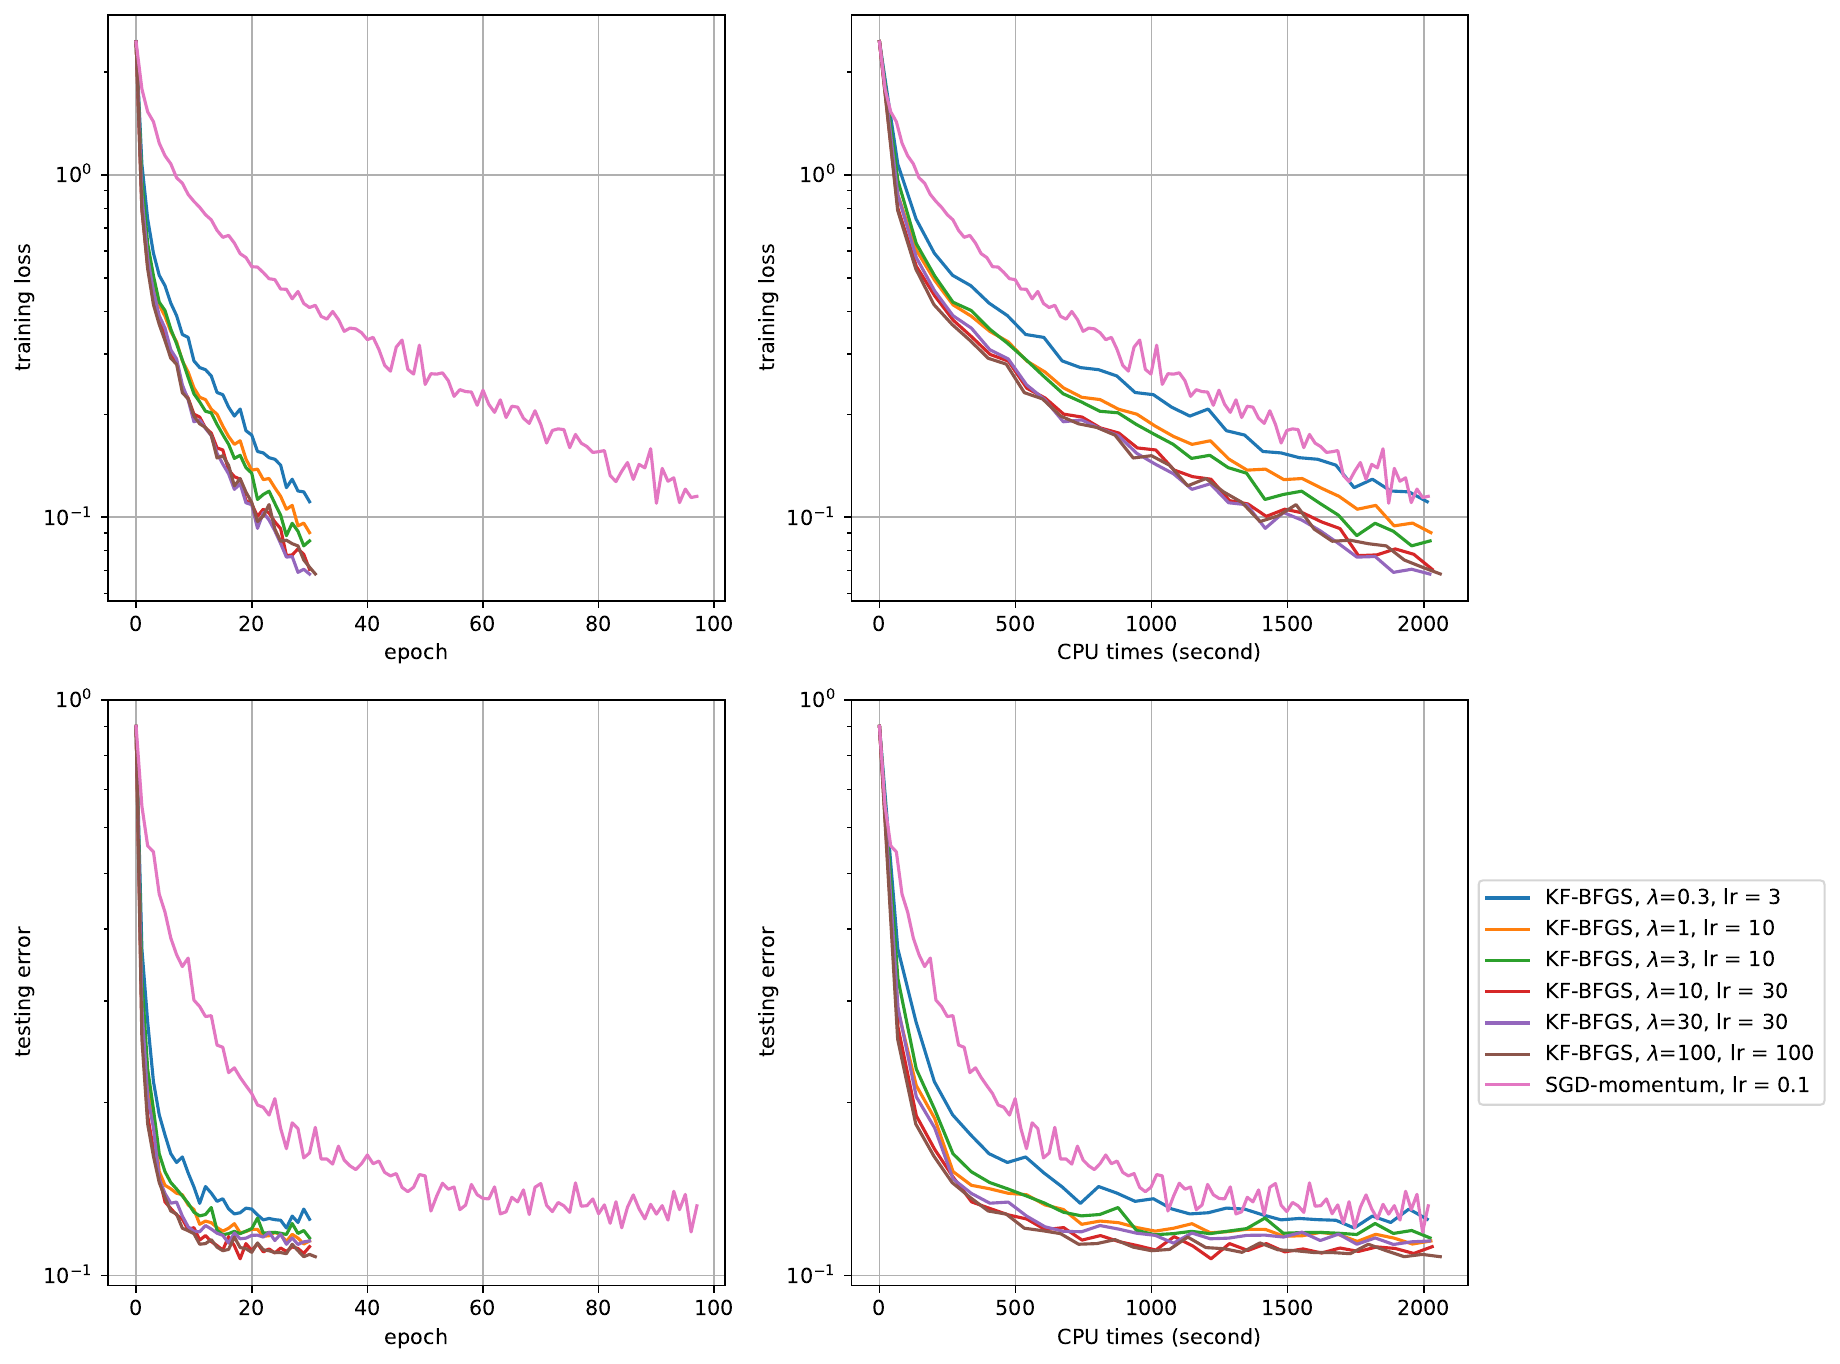}
    \\
    {\footnotesize a) All-CNN model on CIFAR10}
  \end{minipage}
  \begin{minipage}[b]{0.49\textwidth}
    \centering
    \includegraphics[width=\textwidth, height=7cm]{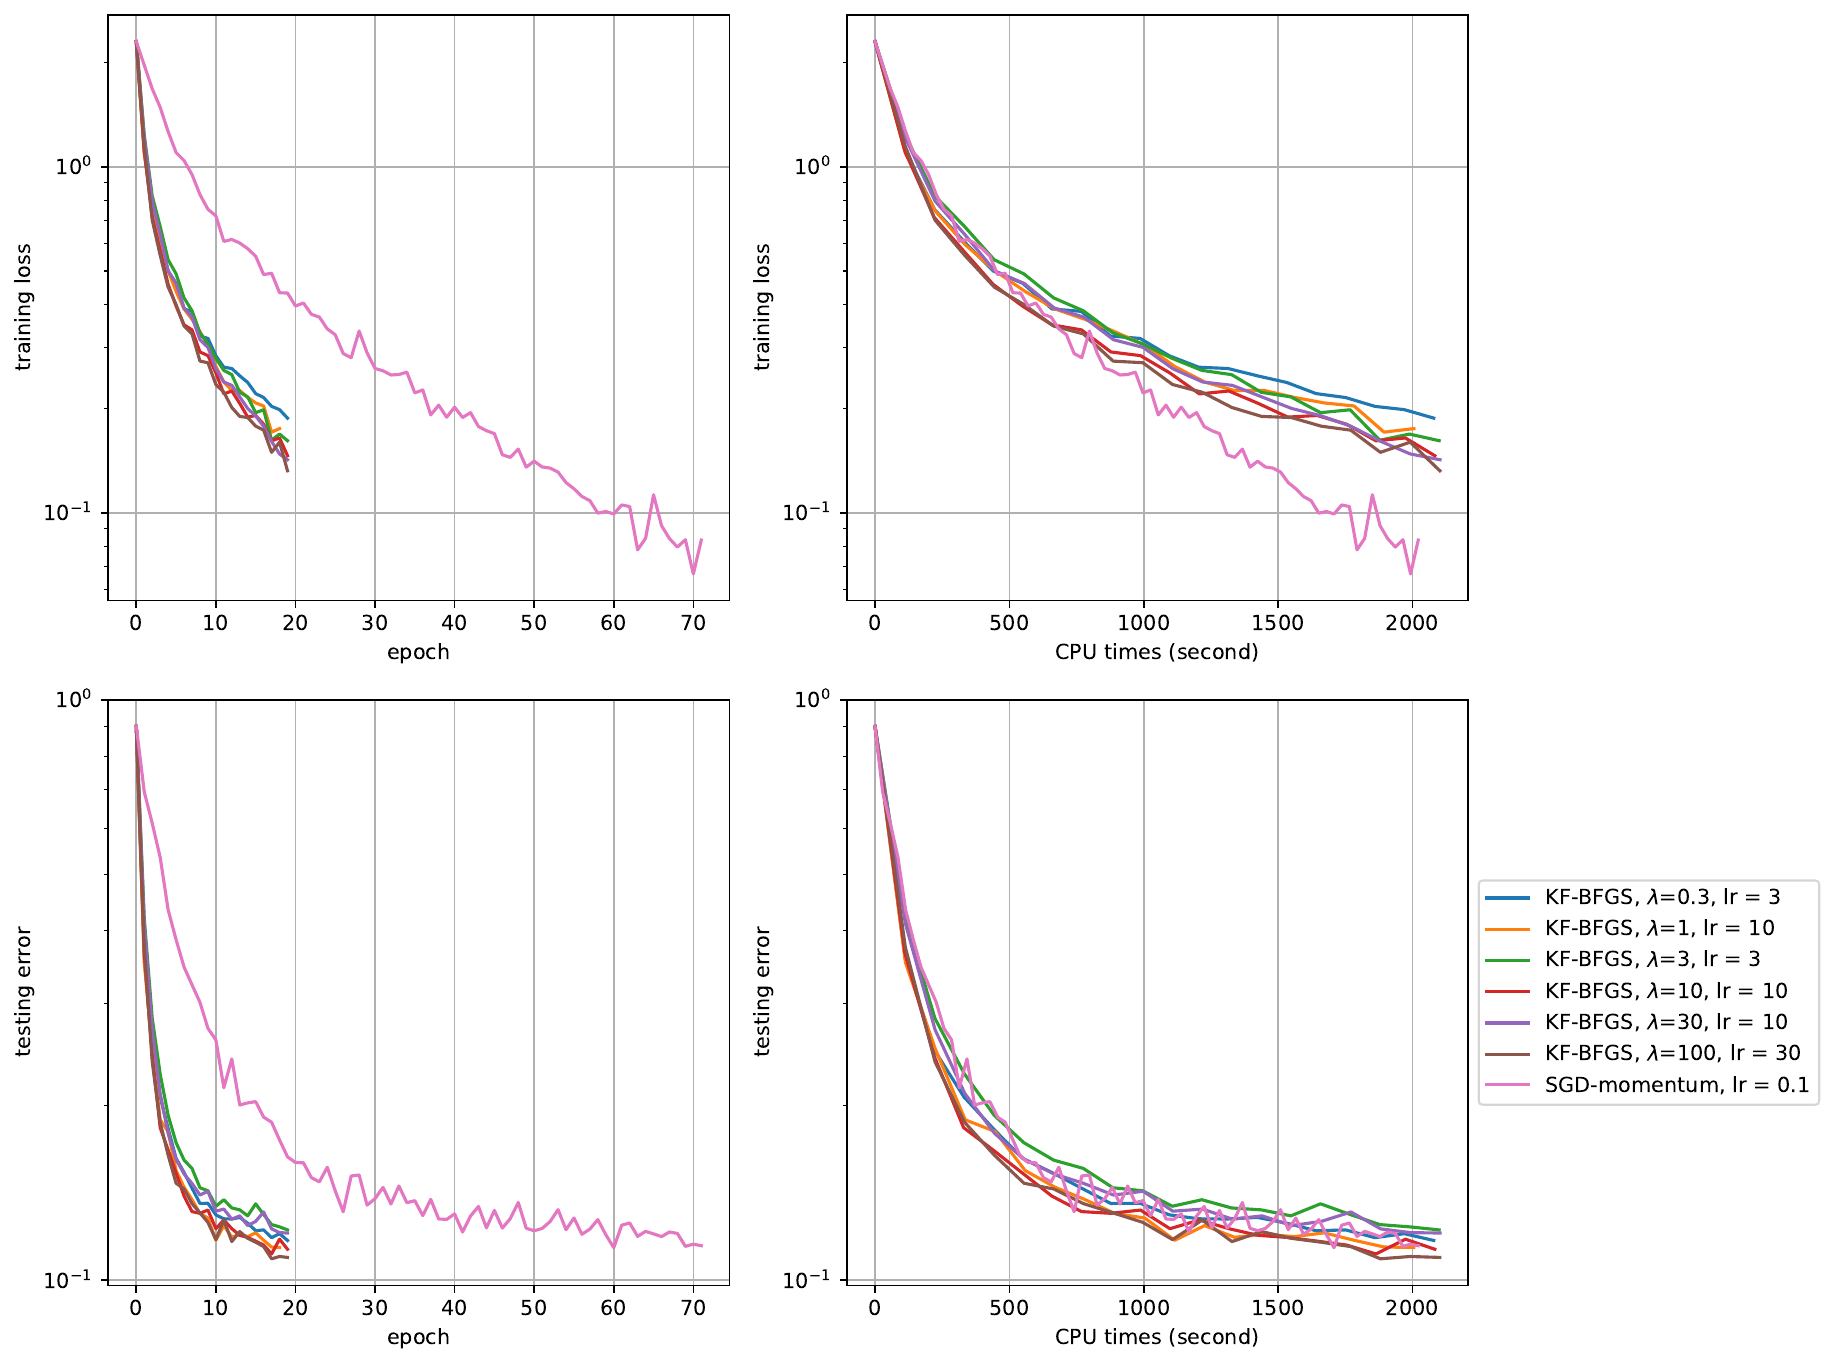}
    \\
    {\footnotesize b) VGG16 model on CIFAR10}
  \end{minipage}
  \begin{minipage}[b]{0.49\textwidth}
    \centering
    \includegraphics[width=\textwidth, height=7cm]{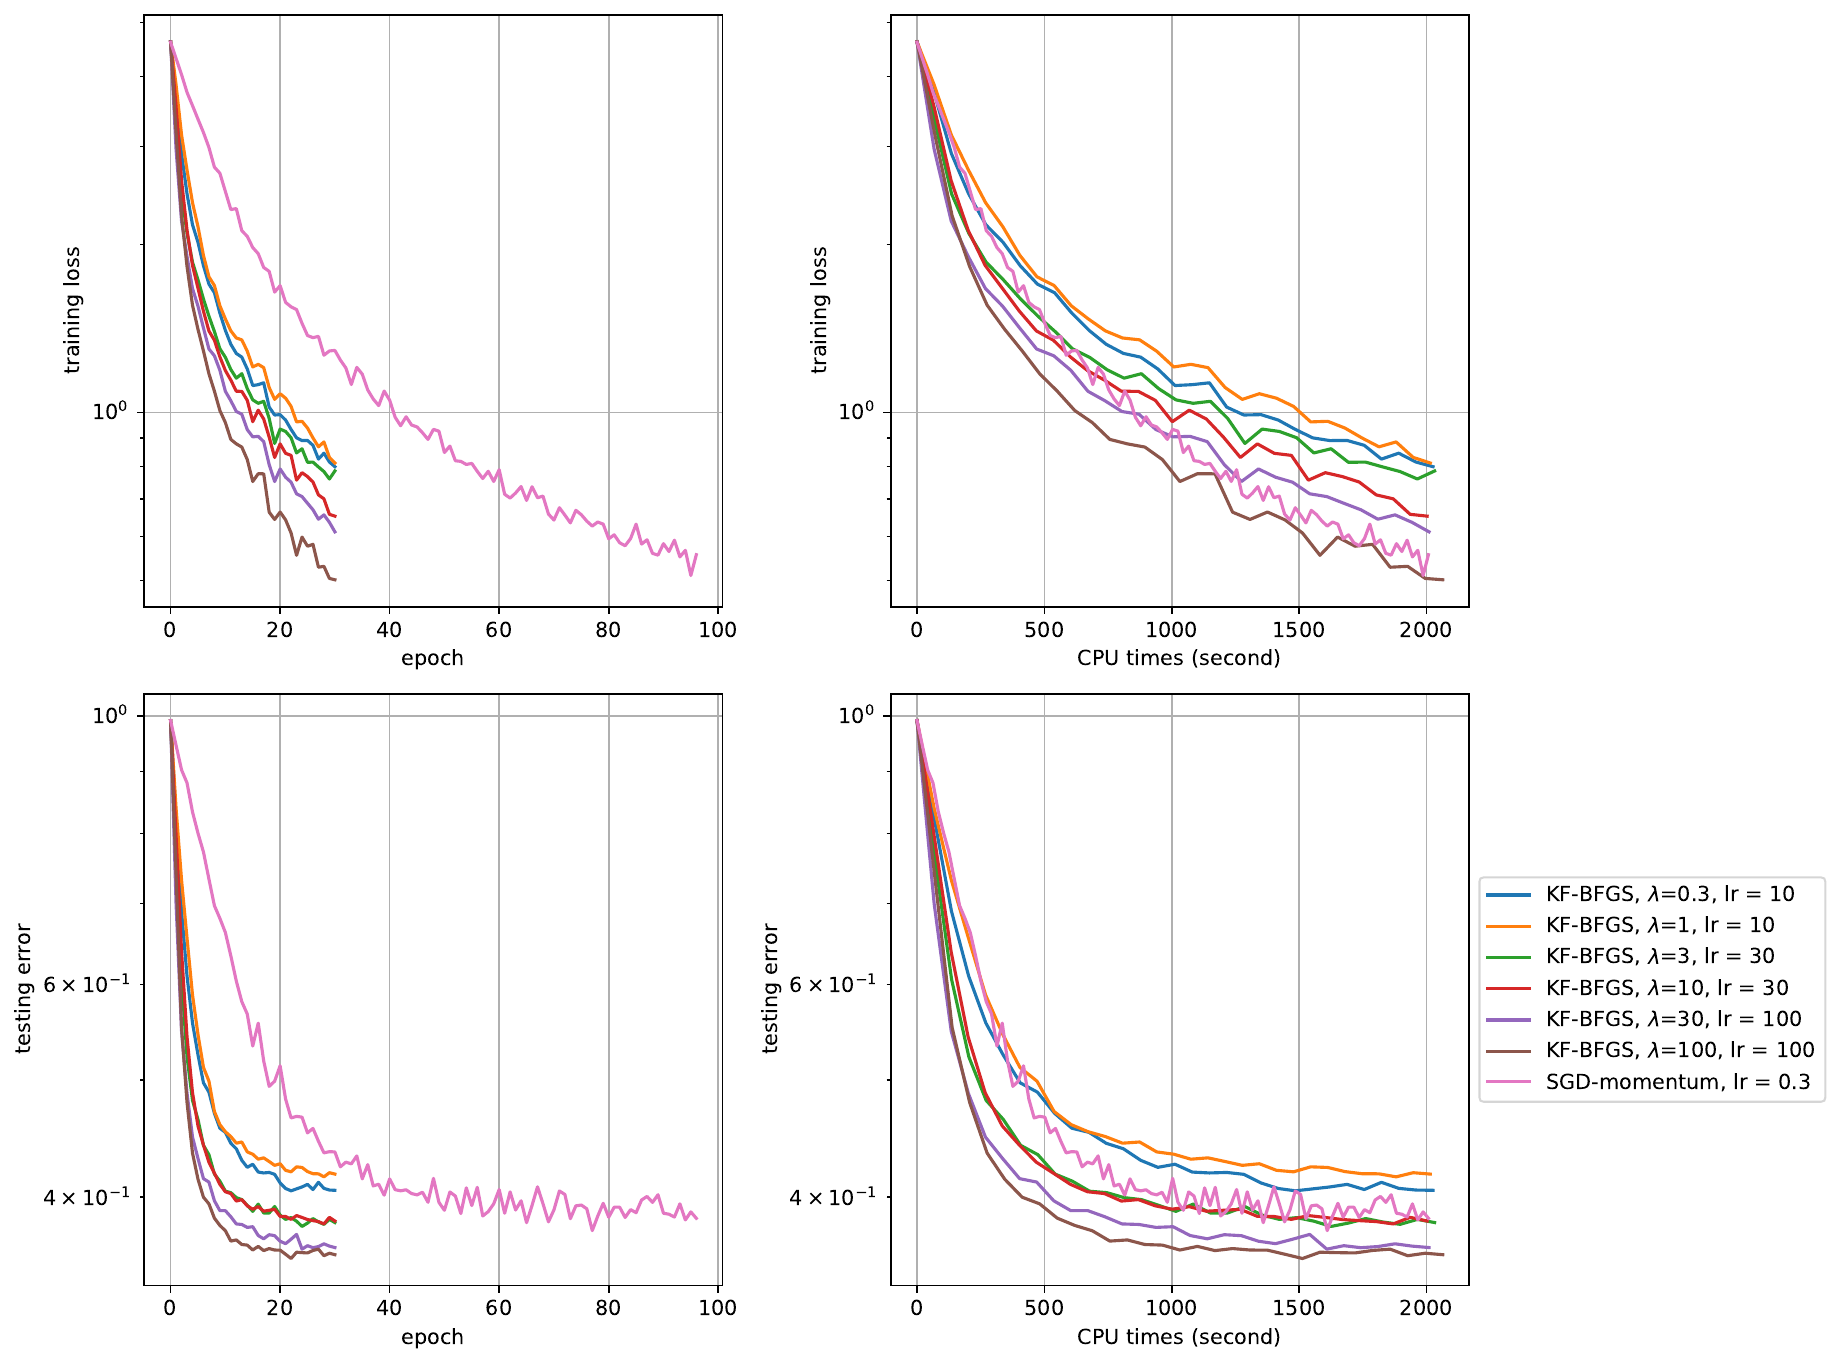}
    \\
    {\footnotesize c) All-CNN model on CIFAR100}
  \end{minipage}
  \begin{minipage}[b]{0.49\textwidth}
    \centering
    \includegraphics[width=\textwidth, height=7cm]{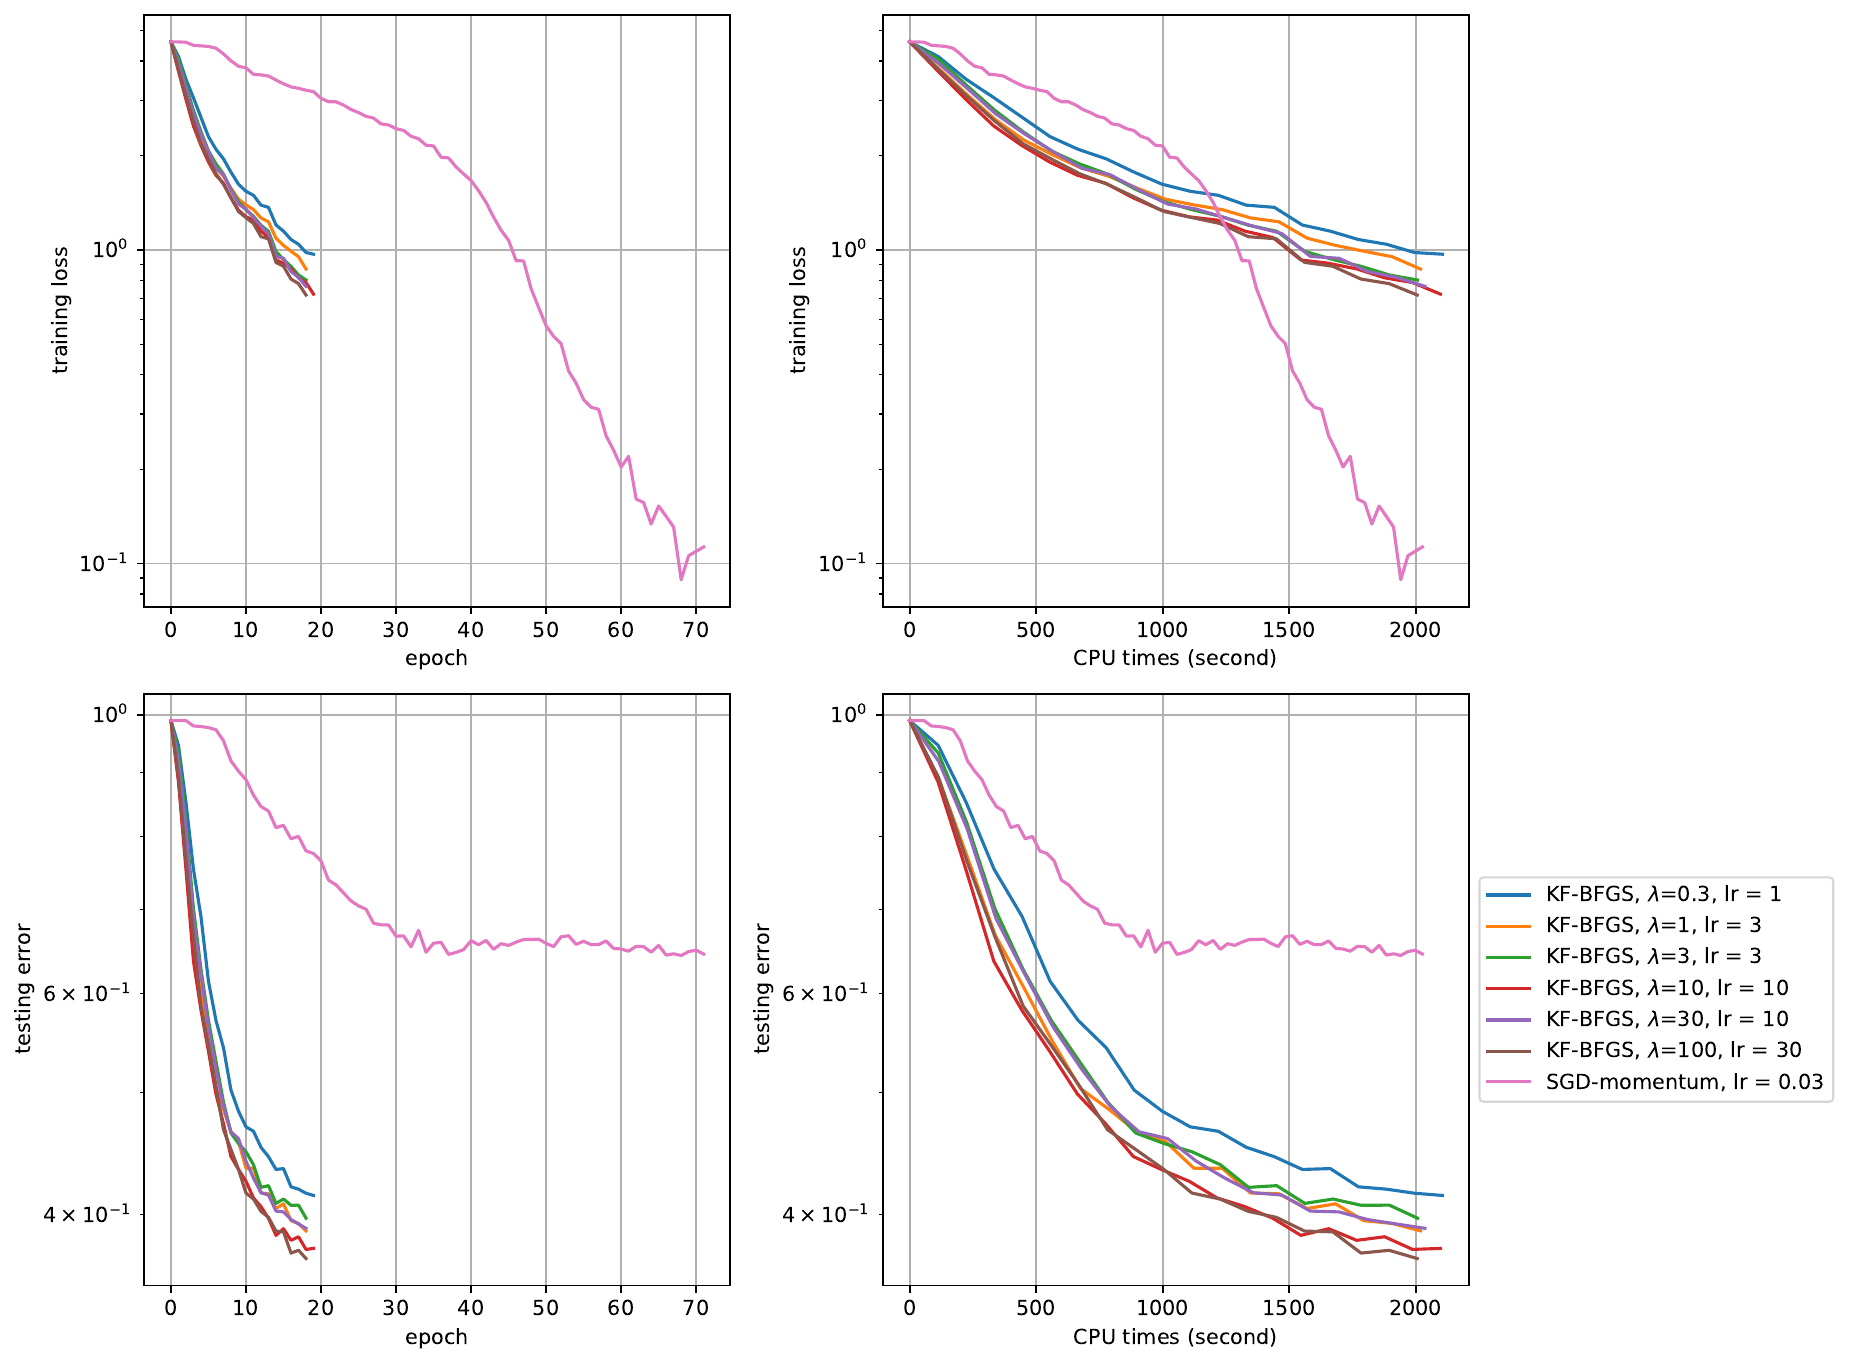}
    \\
    {\footnotesize d) VGG16 model on CIFAR100}
  \end{minipage}

  \caption{
  \clarify{need to update the figures}
  Demonstration of the stability of KF-BFGS-CNN with different HP values (KF-BFGS-CNN is denoted as KF-BFGS in the legend)
  }
  \label{fig_36}
\end{figure*}
