# Supplementary material for: Kronecker-factored Quasi-Newton Methods for Deep Learning
Source: arXiv:2102.06737 source file (2022-02-19)
Supplement: Supplementary file 2 [file proof_not_used.tex]

\addthis{
\begin{lemma}
\clarify{need to add}
\end{lemma}

\begin{proof}

\clarify{need to add subscript A}
Because
\begin{align*}
    || \rho \vs \vs^\top ||
    & = \frac{||\vs||^2}{\vy^\top \vs}
    = \frac{||\vs||^2}{(A \vs + \lambda \vs)^\top \vs}
    = \frac{||\vs||^2}{s^\top A \vs + \lambda ||\vs||^2}
    \\
    & \ge \frac{1}{||A|| + \lambda}.
\end{align*}
we have 
\begin{align*}
    ||H^+||
    & = ||(I - \rho \vs \vy^\top) H (I - \rho \vy \vs^\top) + \rho \vs \vs^\top|| \ge ||\rho \vs \vs^\top|| 
    \\
    & \ge \frac{1}{||A|| + \lambda}.
\end{align*}

On the other hand, because
\begin{align*}
    \rho \vy \vs^\top
    = \frac{(A \vs + \lambda \vs) \vs^\top}{\vs^\top (A \vs + \lambda \vs)}
    = \frac{A \vs \vs^\top + \lambda \vs \vs^\top}{\vs^\top A \vs + \lambda \|\vs\|^2},
\end{align*}
we have 
\begin{align*}
    \| \rho \vy \vs^\top \|
    \ge \frac{\| \lambda \vs \vs^\top \|}{\vs^\top A \vs + \lambda \|\vs\|^2}
    \ge \frac{\lambda \| \vs \vs^\top \|}{(\| A \| + \lambda) \|\vs\|^2}
    = \frac{\lambda}{\| A \| + \lambda},
\end{align*}
\begin{align*}
    \| \rho \vy \vs^\top \|
    & \le \frac{\| A \vs \vs^\top \| + \| \lambda \vs \vs^\top \|}{\vs^\top A \vs + \lambda \|\vs\|^2}
    \le \frac{\| A \| \| \vs \vs^\top \| + \lambda \| \vs \vs^\top \|}{\vs^\top A \vs + \lambda \|\vs\|^2}
    \\
    & \le \frac{\| A \|}{\lambda} + 1.
\end{align*}
Hence, 

\begin{align*}
    \|H^+\| 
    & \leq \|H\| \| I - \rho \vy \vs^\top \|^2 +  \|\frac{\vs \vs^\top}{\vs^\top \vy} \|  
    % \\
    % & \leq\|H\| \Large( \|I\| +  \frac{\|\vs\| \| \vy\|}{\vs^\top \vy}\Large)^2
    %  +  \frac{\vs^\top \vs}{\vs^\top \vy} 
    % \\
    % & \leq (1 + \frac{1}{\sqrt{\mu_2}}\frac{1}{\sqrt{\mu_3}})^2 \|H\| + \frac{1}{\mu_2}.
\end{align*}

\deletethis{
On the other hand, we'd like to prove that $||H|| \le c \lambda^{-1}$ for any iteration $k$. 

Note that this is true at initialization, i.e. $k = 0$. \clarify{how to guarantee this?} Suppose that it is true at iteration $k$. For iteration $k+1$, we'd like to prove that $||H^+|| \le c \lambda^{-1}$.

For any vector $\vx$, we have
\begin{align*}
    & \vx^\top H^+ \vx = \vx^\top \left( (I - \rho \vs \vy^\top) H (I - \rho \vy \vs^\top) + \rho \vs \vs^\top \right) \vx 
    \\
    \le & c \lambda^{-1} ||\vx - \rho \vy (\vs^\top \vx)||^2 + \rho (\vs^\top \vx)^2
    \\
    = & c \lambda^{-1} \left( ||\vx||^2 + ||\rho \vy (\vs^\top \vx)||^2 - 2 \rho (\vx^\top \vy) (\vs^\top \vx) \right) + \rho (\vs^\top \vx)^2
\end{align*}
Thus,
\begin{align}
    & \vx^\top H^+ \vx \le c \lambda^{-1} ||\vx||^2
    \\
    \Leftrightarrow
    & c \lambda^{-1} \left( \rho (\vs^\top \vx) || \vy ||^2 - 2 (\vx^\top \vy) \right) + (\vs^\top \vx) \le 0
    \\
    \Leftrightarrow
    & c \lambda^{-1} \left( (\vs^\top \vx) || \vy ||^2 - 2 (\vx^\top \vy) (\vs^\top \vy) \right) + (\vs^\top \vx) (\vs^\top \vy) \le 0
    \\
    \Leftrightarrow
    & (\vs^\top \vx) || \vy ||^2 - 2 (\vx^\top \vy) (\vs^\top \vy) + c^{-1} \lambda (\vs^\top \vx) (\vs^\top \vy) \le 0
    \\
    \Leftrightarrow
    & (\vs^\top \vx) || \vy ||^2 \le (\vx^\top (2 \vy - c^{-1} \lambda \vs)) (\vs^\top \vy)
    \label{eq_17}
\end{align}

% \ref{eq_16}
% \ref{eq_17} no

Because $\vy = A \vs + \lambda \vs$,
\begin{align*}
    & (\ref{eq_17})
    \\
    \Leftrightarrow
    & (\vs^\top \vx) || A \vs + \lambda \vs ||^2 
    \\
    \le & (\vx^\top (2 A \vs + (2-c^{-1}) \lambda \vs)) (\vs^\top (A \vs + \lambda \vs))
    \\
    \Leftrightarrow
    & (\vs^\top \vx) (\vs^\top A^2 \vs + \lambda^2 || \vs ||^2 + 2 \lambda \vs^\top A \vs)
    \\
    \le & (2 \vx^\top A \vs + (2-c^{-1}) \lambda (\vx^\top \vs)) (\vs^\top A \vs + \lambda ||\vs||^2)
\end{align*}
}

\end{proof}
}
